# Supplementary material for: A continuum theory of phase separation kinetics for active Brownian particles
Source: arXiv:1307.4373 ancillary file (2013-10-03)
Supplement: Supplementary file 1 [file SM.pdf]

# A continuum theory of phase separation kinetics for active Brownian particles
# Supplemental Material

Joakim Stenhammar,* Adriano Tiribocchi, Rosalind J. Allen, Davide Marenduzzo, and Michael E. Cates
*SUPA, School of Physics and Astronomy, University of Edinburgh,*
*JCMB Kings Buildings, Edinburgh EH9 3JZ, United Kingdom*

## PHASE DIAGRAM

In Fig. S1, the phase diagram in the $\phi - \mathrm{Pe}$ plane obtained from ABP simulations is shown. The approximate phase boundary was determined from assessing the parameters for which $L(t)$ exhibited a persistent coarsening over time. While the onset of phase separation was found to be very distinct when moving along the $\phi$-axis, the phase boundary in the Pe-direction is more diffuse. The phase diagram is in broad agreement with that determined in Ref. [1].

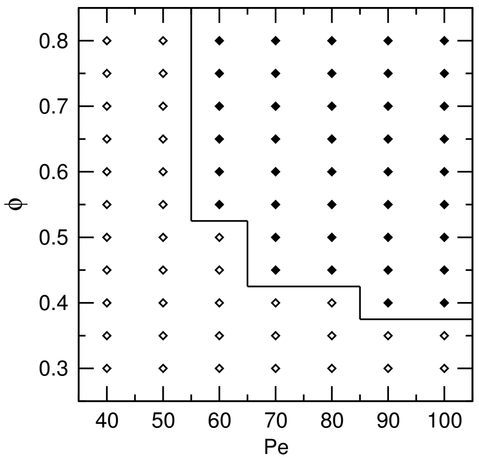


Figure S1. Phase diagram as a function of the particle area fraction $\phi$ and Péclet number Pe, obtained from simulations of ABP fluids. Filled symbols denote state points with a gas-liquid coexistence, whereas empty symbols indicate a homogeneous suspension.

## COMMON-TANGENT CONSTRUCTION ON BULK FREE ENERGY

In Figure S2, we plot the bulk free energy density $f = f_0 + f_{\mathrm{rep}}$ resulting from the continuum theory [Eqs. (3) and (7)] with the choice of $v(\phi)$ motivated in the main text. From the usual common-tangent construction on $f$ (dashed line in Figure S2), this is expected to lead to two coexisting phases with area fractions $\phi_1 \approx 0.28$ and $\phi_2 \approx 0.93$; as was shown in Fig. 4, this result is in good correspondence with results from numerical simulations. However, as is also clear from Fig. S2, the densities of both coexisting phases will be affected by the exact form of the repulsive potential, and thus a quantitative correspondence with those observed in ABP simulations cannot be expected; attempts to improve this by varying $k_{\mathrm{rep}}$ and $\phi_{\mathrm{t}}$ are frustrated by the $\ln(1-\phi)$ term in Eq. (10), which introduces a numerical instability as $\phi \to 1$.

The details of $f_{\mathrm{rep}}$ will also affect the precise location of the binodals (which are anyway very hard to determine directly from ABP simulations because phase nucleation becomes slow as they are approached). In addition, the interesting structure in the kinetic phase diagram (Fig. S1) arises at the low Pe end, where the mapping behind $f_0$ must ultimately fail as thermal Brownian diffusion takes over [2]. Thus we cannot connect $v(\phi)$ and $f_{\mathrm{rep}}$ closely enough to the microscopic ABP variables (Pe and the interparticle potential) to account quantitatively for the phase boundaries. To achieve this, a microscopic theory with Pe directly as the control parameter is better suited, along lines used successfully in Ref. [1], although this gives no account of phase separation kinetics. Nonetheless we can obtain quantitative agreement in dynamics, at least for deep quenches as studied here.

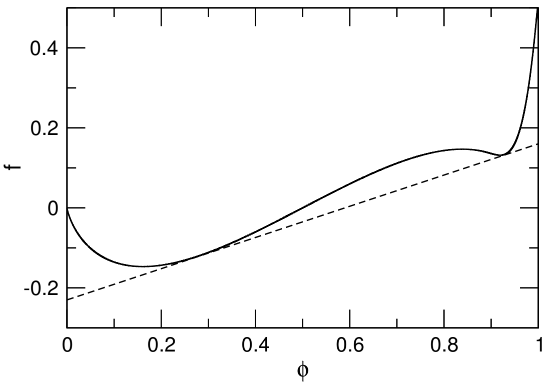


Figure S2. Bulk free energy density $f = f_0 + f_{\mathrm{rep}}$ obtained using $v(\phi) = (1-\phi)$, $\phi_{\mathrm{t}} = 0.88$, and $k_{\mathrm{rep}} = 2500$. Terms linear in $\phi$ have been subtracted for clarity. The dashed line represents a common-tangent construction on $f$, indicating the approximate coexistence densities $\phi_1 \approx 0.28$ and $\phi_2 \approx 0.93$.

## Pe-DEPENDENCE OF SWIM SPEED

In Fig. S3, the density-dependent swim speed $v(\phi)$ for three different values of Pe is shown. Clearly, the dependence of $v(\phi)$ on Pe is weak throughout the range $40 \leq \text{Pe} \leq 100$ considered, as long as $v$ is sampled within the one-phase region. In the phase-separated region, the measured $v(\phi)$ constitutes a weighted average over the two phases and thus becomes significantly different. It should however be emphasized that it is the $v(\phi)$ from the *homogeneous* system that should be used for deriving $\mu$, and we can thus safely assume that the $v(\phi)$ and $D(\phi)$ obtained from the (homogeneous) Pe = 40 system are transferable to the (phase-separated) Pe = 100 case.

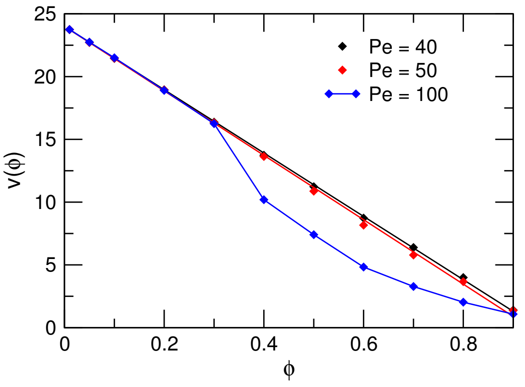


Figure S3. Effective swim speed $v(\phi)$ as a function of the area fraction $\phi$ at different values of Pe, as indicated. The black and red solid lines are fits to the respective data points of the function $v(\phi) = v_0(1-a\phi)$, with the optimized values $a = 1.05$ (Pe = 40) and $a = 1.07$ (Pe = 50). The blue solid line is a guide to the eye. The observed deviation from linearity for $\phi \geq 0.4$ in the Pe = 100 system is due to the onset of phase separation, in accordance with the phase boundary in Fig. S1.

## SIMULATION DETAILS

The continuum equations [Eqs. (10) – (13)] were solved numerically using a standard Euler finite-difference scheme using the parameter values $k_{\text{rep}} = 2500$, $\phi_{\text{t}} = 0.88$, and $\kappa_0 = 0.3$. For comparison with ABP simulations, a lattice size of $150^2$ $[(60\lambda)^2]$ was employed, whereas a lattice size of $512^2$ was used for the calculation of the growth exponent. A mesh size of $0.4\lambda$ and a timestep of $5 \times 10^{-3}\tau_{\text{r}}$ was used throughout, and periodic boundary conditions were applied. The initial condition was taken to be one of uniform density, with a local random offset of $\approx 5\%$.

The microscopic ABP model consists of spherical particles interacting pairwise through a repulsive Weeks-Chandler-Andersen potential, given by $U = 4\varepsilon\left[(\sigma/r)^{12} - (\sigma/r)^6\right] + \varepsilon$ if $r < 2^{1/6}\sigma$, and $U = 0$ otherwise. Here $\sigma$ denotes the particle diameter, $\varepsilon$ determines the interaction strength, and $r$ is the center-to-center separation between two particles. The model was studied by solving the fully overdamped translational and rotational Langevin equations

$$\partial_t \mathbf{r}_i = \beta D_{\text{t}}\left[\mathbf{F}_i + F_{\text{p}}\mathbf{p}_i\right] + \sqrt{2D_{\text{t}}}\boldsymbol{\Lambda}_{\mathbf{r}} \quad \text{(S1)}$$

$$\partial_t \theta_i = \sqrt{2D_{\text{r}}}\Lambda_\theta, \quad \text{(S2)}$$

where $\mathbf{F}_i$ is the total conservative force on particle $i$, $F_{\text{p}}$ is the (constant) magnitude of the self-propulsion force, whose direction is defined by $\mathbf{p}_i = (\cos\theta_i, \sin\theta_i)$, $D_{\text{t}}$ and $D_{\text{r}} = 3D_{\text{t}}/\sigma^2$ denote the translational and rotational diffusivities, $\beta = (k_{\text{B}}T)^{-1}$ is the inverse thermal energy, and $\boldsymbol{\Lambda}_{\mathbf{r}}$ and $\Lambda_\theta$ are random variables as discussed following Eq. (1). Eqs. (S1)–(S2) were solved using a slightly modified version of the LAMMPS [3] molecular dynamics software package. Periodic boundary conditions were applied throughout. For determining the phase diagram, a system of side length $L_x = L_y = 150\sigma$ ($N \approx 20000$ particles) was used, whereas larger systems with $L_x = L_y = 1000\sigma$ ($N \approx 700000$) were used for studying the phase separation kinetics (where Pe was kept constant at Pe = 100). In terms of Lennard-Jones time units $\tau_{\text{LJ}} = \sigma^2/(\varepsilon\beta D_{\text{t}})$, a time step of $5 \times 10^{-5}\tau_{\text{LJ}}$ was used, and each simulation was run for $10^8$ timesteps, amounting to $\sim 90$ hours of computing time on a 2048-core IBM Blue Gene/Q node. While the microscopic model is essentially identical to that studied in Ref. [1], there is a subtle difference in that we varied Pe through varying $D_{\text{t}}$ (in practice, by varying the temperature), while keeping $F_{\text{p}}$, and thus $v_0$, constant at a value of $F_{\text{p}} = 24\varepsilon/\sigma$. All simulations were started from an initial configuration of equilibrated passive colloids ($F_{\text{p}} = 0$) with $k_{\text{B}}T = \varepsilon$, by switching on $F_{\text{p}}$ at $t = 0$. In terms of Lennard-Jones units, the reduced length and time scales in the ABP systems with Pe = 100 are given by $\lambda = 16.67\sigma$ and $\tau_{\text{r}} = 1.389\tau_{\text{LJ}}$; the former mapping furthermore leads to $N_0 = 4\lambda^2/(\pi\sigma^2) \approx 354$, which was used to set the noise strength when numerically solving Eq. (13).

As our operational microscopic definition of $v(\phi)$, we chose the average of the instantaneous velocities of all particles projected onto their self propulsion direction:

$$v = \beta D_{\text{t}}\langle(F_{\text{p}}\mathbf{p}_i + \mathbf{F}_i)\cdot\mathbf{p}_i\rangle \quad \text{(S3)}$$

Note that $v = \beta D_{\text{t}} F_{\text{p}} = v_0$ in the limit $\phi \to 0$, where interparticle forces become negligible. Finally, the density-dependent effective diffusivity $D(\phi)$ was independently measured by linear fitting to the long-time limit of the mean-square displacement $\langle R^2\rangle = 4Dt$. To ensure a reasonably homogeneous density, $v$ and $D$ were measured on systems just outside the two-phase region, at Pe = 40.

The characteristic domain scale $L(t)$ was computed as the inverse of the first moment of the static structure

factor $S(k,t)$

$$L(t) = 2\pi \left[ \frac{\int_{2\pi/L}^{k_{\rm cut}} k S(k,t) \mathrm{d}k}{\int_{2\pi/L}^{k_{\rm cut}} S(k,t) \mathrm{d}k} \right]^{-1}, \tag{S4}$$

where $L$ is the length of the simulation box and the upper cut-off $k_{\rm cut}$ was taken to be the first minimum in $S(k)$.

Snapshots from ABP simulations (Fig. 1) were obtained by coarse-graining the local density on a grid with size $256^2$, using a weighting function $w(r) \sim \exp\left[-r_{\rm cut}^2/(r_{\rm cut}^2 - r^2)\right]$, where $r$ is the distance of a particle from the a particular lattice point, and $r_{\rm cut} = \sqrt{2}L/256$ was chosen as the cut-off distance where $w(r) \to 0$.

## MOVIES

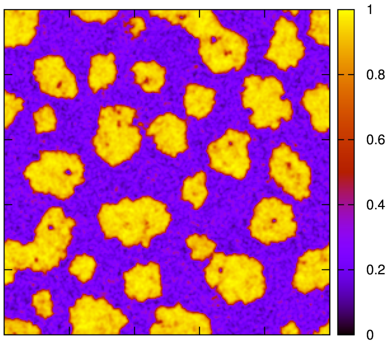


Figure S4. **abp_0.5.mp4** Video showing domain coarsening in an ABP system at area fraction $\phi = 0.5$. The temporal separation between frames is $7.2\tau_{\rm r}$, with 25 frames per second.

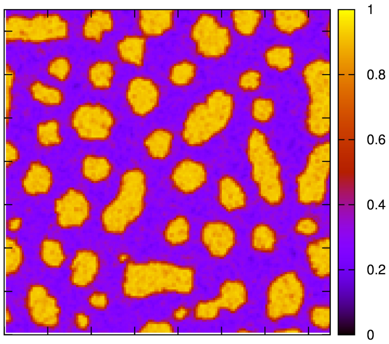


Figure S5. **cont_0.5.mp4** Video showing domain coarsening as obtained by solving Eq. (13) with average area fraction $\phi = 0.5$. The temporal separation between frames is $7.2\tau_{\rm r}$, with 25 frames per second.

* j.stenhammar@ed.ac.uk

[1] G. S. Redner, M. F. Hagan, and A. Baskaran, Phys. Rev. Lett. **110**, 055701 (2013).
[2] M. E. Cates and J. Tailleur, EPL **101**, 20010 (2013).
[3] S. Plimpton, J. Comp. Phys. **117**, 1 (1995).
